# Supplementary material for: Neutron valence structure from nuclear deep inelastic scattering
Source: arXiv:1908.02223 ancillary file (2020-04-21)
Supplement: Supplementary file 1 [file Supplementary_v0.pdf]

# Supplementary Materials: Neutron valence structure from nuclear deep inelastic scattering

## MODEL DERIVATION

Taking all of the modification of  $F_2^A$  to be when nucleons are in an np-SRC configuration (neglecting nn and pp contributions) and self-consistently using  $F_2^d$  to get to  $F_2^n$ :

$$\begin{aligned} F_2^A &= (Z - n_{SRC}^A)F_2^p + (N - n_{SRC}^A)F_2^n + n_{SRC}^A(F_2^{p*} + F_2^{n*}) \\ F_2^A &= ZF_2^p + NF_2^n + n_{SRC}^A(\Delta F_2^p + \Delta F_2^n) \\ F_2^n &= F_2^d - F_2^p - n_{SRC}^d(\Delta F_2^p + \Delta F_2^n) \end{aligned} \quad (1)$$

To compare to EMC ratio data, we can write this as:

$$\frac{2F_2^A}{AF_2^d} = \frac{2N}{A} + \frac{2(Z - N)}{A} \frac{F_2^p}{F_2^d} + \left( \frac{2n_{SRC}^A}{An_{SRC}^d} - \frac{2N}{A} \right) \frac{n_{SRC}^d(\Delta F_2^p + \Delta F_2^n)}{F_2^d} \quad (2)$$

where in this model, we define  $a_2^A \equiv 2n_{SRC}^A/An_{SRC}^d$ . Eqn. 2 is highly nucleus-dependent, except for the universal term,  $f_{\text{univ}} = n_{SRC}^d(\Delta F_2^p + \Delta F_2^n)/F_2^d$ . Ref [1] used measurements of  $a_2^A$  and a parameterization of  $F_2^p/F_2^d$  in order to solve for  $f_{\text{univ}}(x)$  using EMC ratio data points,  $2F_2^A/AF_2^d$ . In this work, we expanded on that analysis to do a global extraction of  $f_{\text{univ}}$ ,  $F_2^p/F_2^d$ , and  $a_2^A$  (as well as nuisance parameters related to each data set of  $2F_2^A/AF_2^d$ ).

## UNIVERSAL FUNCTION EXTRACTION

To model the universal function and  $F_2^p/F_2^d$ , we chose parameterizations:  $f_{\text{univ}} = \alpha + \beta x + \gamma e^{\delta(1-x)}$ ,  $F_2^p/F_2^d \equiv R_{pd}(x) = \alpha_{pd} + \beta_{pd} + \gamma_{pd}e^{\delta_{pd}(1-x)}$ , which are robust enough to characterize EMC-type curves. We developed a generative Bayesian model and performed inference of our model parameters using the Hamiltonian Markov Chain Monte Carlo package, PyStan [2, 3].

Given our model and world EMC data, we construct the following likelihood that PyStan uses when sampling the posterior distribution of our model:

$$\begin{aligned} \left( \frac{2F_2^A}{AF_2^d} \right)_i &\sim \text{norm} \left\{ s_i \cdot \left[ \frac{2(A - Z)}{A} + \frac{2(2Z - A)}{A} R_{pd}(x) + \left( a_2^A - \frac{2(A - Z)}{A} \right) f_{\text{univ}}(x) \right], \delta_i \right\} \\ \left( \frac{F_2^p}{F_2^d} \right) &\sim \text{norm} \left\{ s_{pd} \cdot R_{pd}(x), \delta \right\} \end{aligned} \quad (3)$$

where  $(2F_2^A/AF_2^d)_i$  is an EMC-ratio measurement series of nucleus  $(A, Z)$  with point-to-point uncertainties  $\delta_i$  (there can be multiple series for a given nucleus). The only parameter unique to this series is  $s_i$ , which is a nuisance normalization parameter that allows the model to re-scale the EMC-ratio series. The parameter  $a_2^A$  is only unique to this series  $i$  if it is the only series for that nucleus  $(A, Z)$ , otherwise it is shared when inputting multiple measurements of the same nucleus. The four parameters of  $R_{pd}(x)$  are constrained in every EMC-ratio series, as well as the independent data of  $(F_2^p/F_2^d)$ , which has point-to-point uncertainties  $\delta$  and is allowed to also have a re-scaling given by the parameter  $s_{pd}$ .

The only priors used in our model are that (1) the parameter  $a_2^A$  follow a normal distribution around the measured  $a_2^A$  with a standard deviation given by the experimental uncertainty, and (2) the scaling parameters  $s_i, s_{pd}$  follow a normal distribution around one with a standard deviation given by the experimental normalization uncertainty.

# QUALITY OF MODEL EXTRACTION

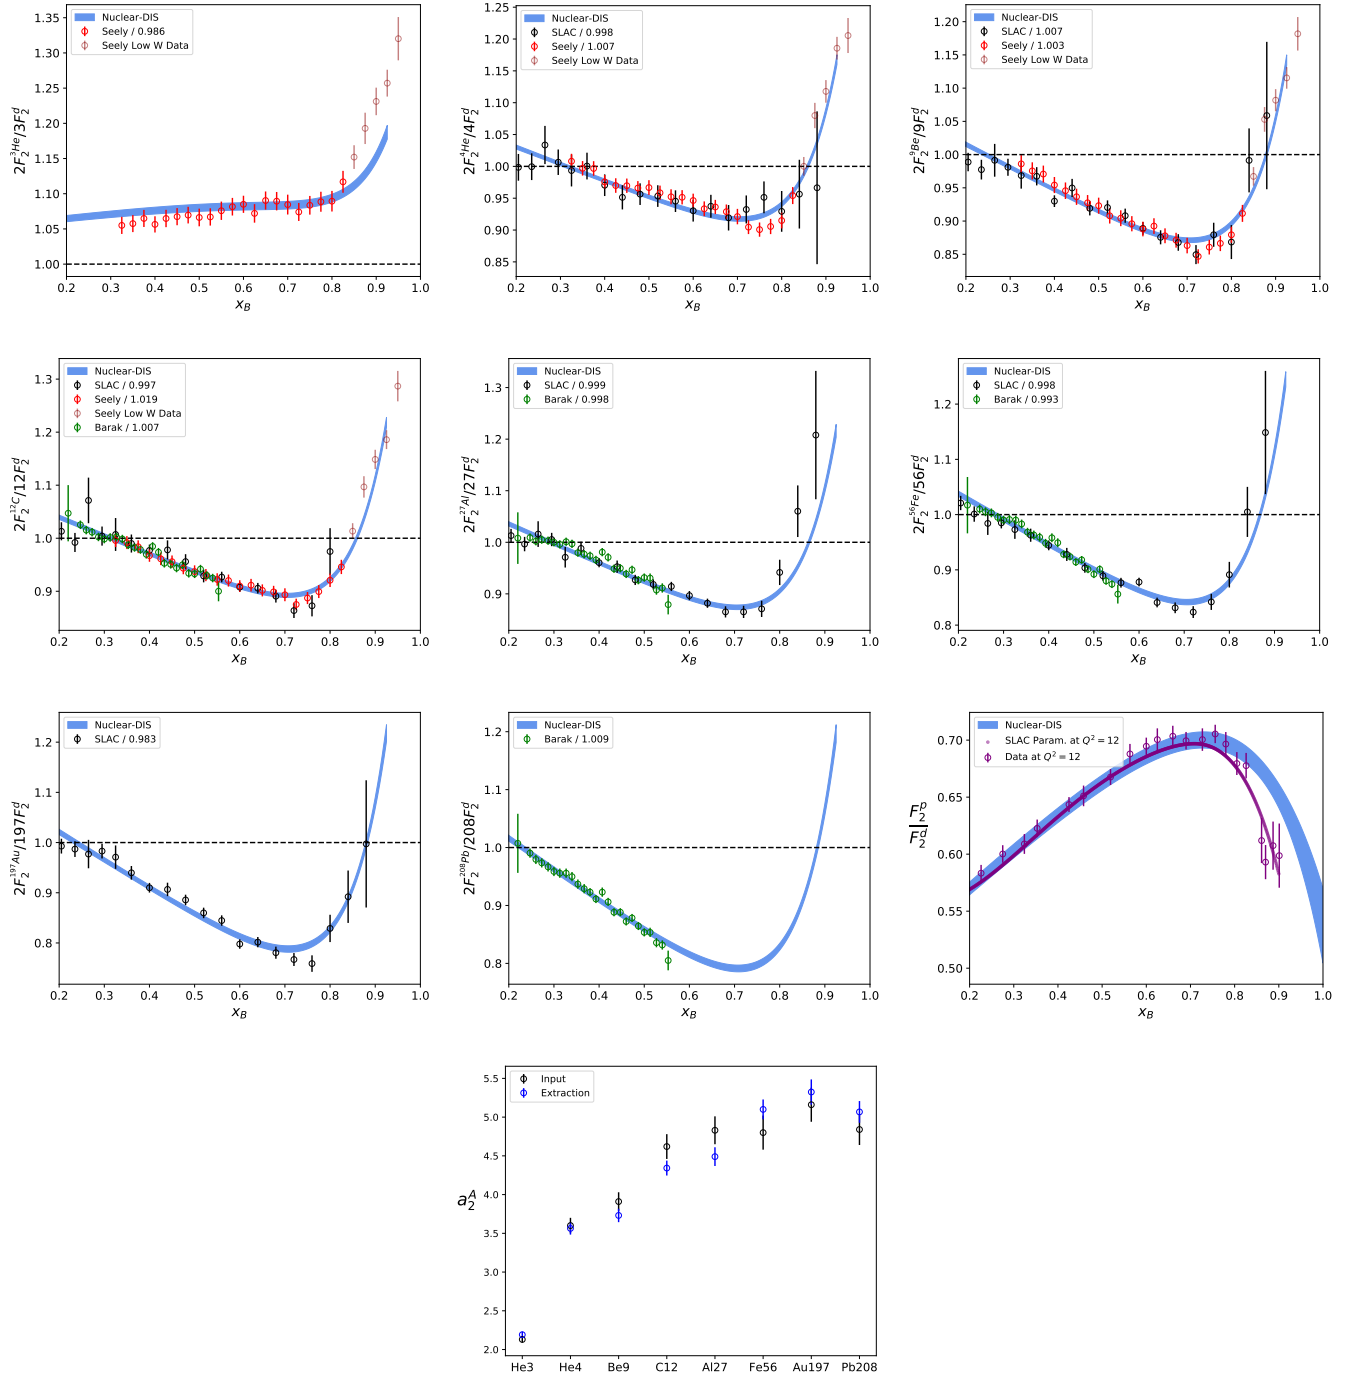

FIG. 1: Global extraction model with 68% bands compared to all input data provided to model. All Seely data [4] were used in the fitting, and  $F_2^p/F_2^d$  data was kept at  $Q^2 = 12 \text{ GeV}^2$  from Arrington et al. [5]

## POSTERIOR PARAMETER SAMPLES

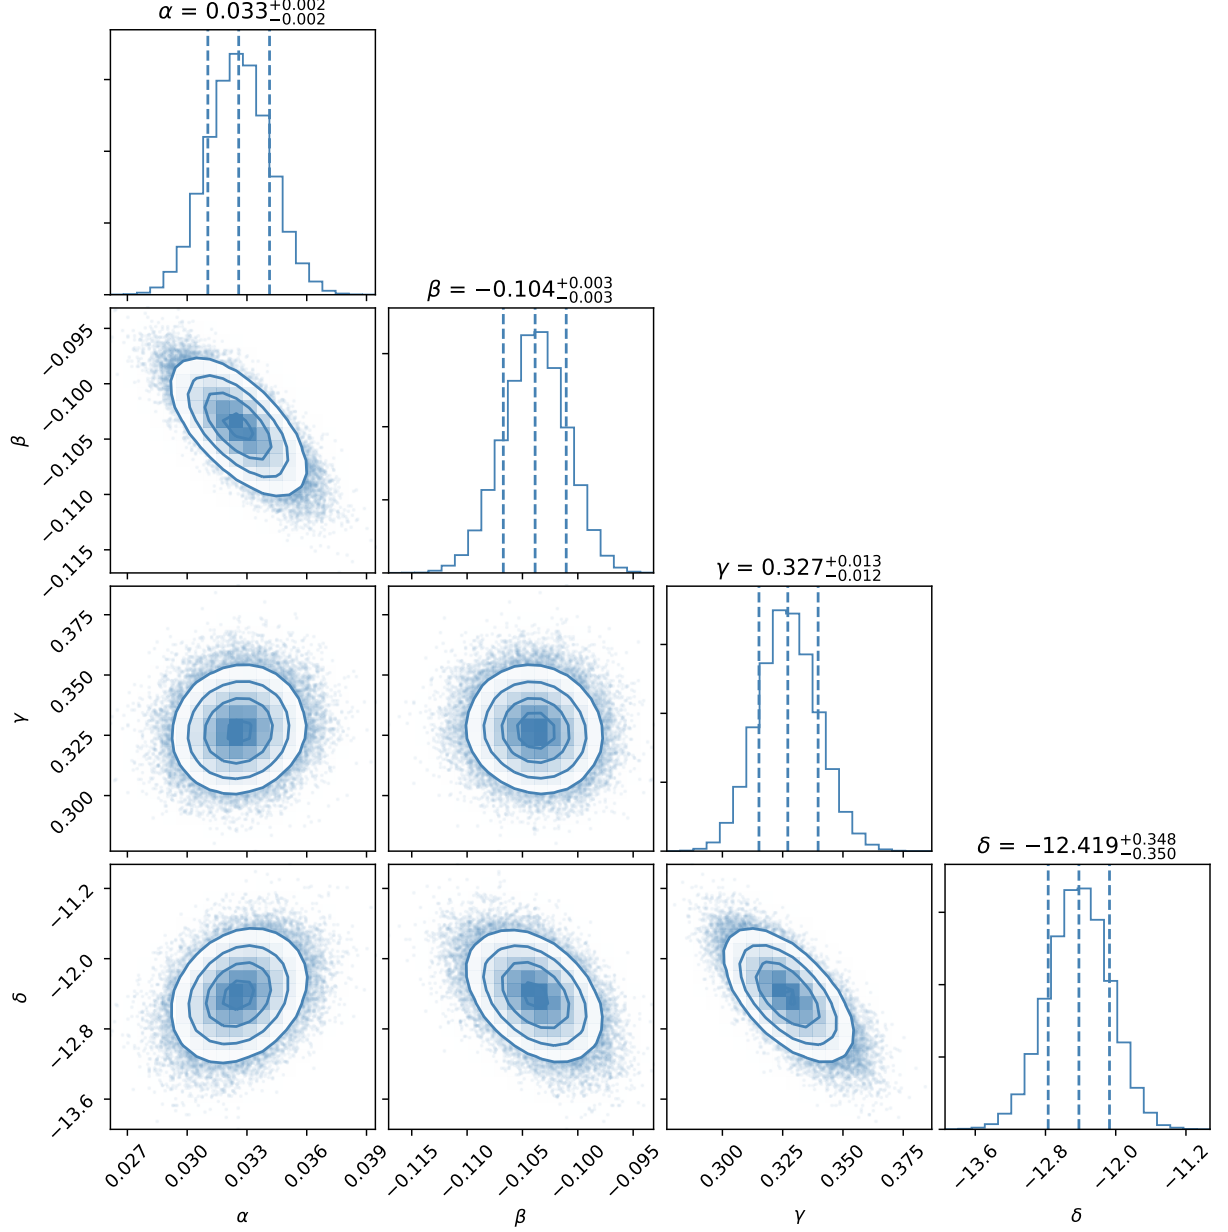

FIG. 2: Correlation matrix of the parameters of our universal function. On the diagonal are 1D distributions of each parameter, showing the most likely value for that parameter. Each off-diagonal plot is then a correlation plot between two parameters. The full 31 parameter space ( $\alpha, \beta, \gamma, \delta$  for the universal function  $f_{\text{univ}}$ ,  $\alpha_d, \beta_d, \gamma_d, \delta_d$  for  $R_{pd}(x)$ ,  $s_d$  for the normalization re-scaling parameter for the input data set of  $R_{pd}$ , each extracted  $a_2$  for all nuclei used as input, and all normalization re-scaling parameters for each data set used as input) can be accessed via the supplied text file with the supplementary materials. The posterior prefers the measured  $^3\text{He}$  EMC ratio [4] be re-scaled by about 2%, which is at the higher end of its normalization uncertainty and consistent with the independent renormalization of Ref. [6].

## LOW $W^2$ , HIGH $x_B$ DATA; $Q^2$ DEPENDENCE

The data used in this analysis were measured at varying values of invariant hadronic mass,  $W$ , and  $Q^2$ . For  $W^2 > 2$  GeV<sup>2</sup> and  $Q^2 > 2$  GeV<sup>2</sup>, the ratio  $F_2^A/F_2^d$  was shown to be largely insensitive to higher twist effects, as evident by its  $Q^2$  independence [1, 4, 7, 8]. The extracted UMF extends up to  $x_B \sim 0.95$ . As discussed below, for  $x_B > 0.8$  the available data is primarily at  $W^2 < 2$  GeV<sup>2</sup>, well below the deep inelastic region [8]. In addition, at  $x_B \geq 0.9$ , the experimental data is less accurate and likely more  $Q^2$ -dependent, in particular due to quasi-elastic contamination. At  $x_B \geq 0.8$ , where the data are predominantly at  $W^2 < 2$  GeV<sup>2</sup>, this  $Q^2$ -independence was demonstrated over a smaller range. We therefore assume that  $F_2^A/F_2^d$  is  $Q^2$ -independent, but indicate the region of  $x_B > 0.8$  which includes the low  $W^2$  data. Lastly, as  $F_2^p/F_2^d$  does show some  $Q^2$  dependence, the input data of  $F_2^p/F_2^d$  is extracted at  $Q_0^2 = 12$  GeV<sup>2</sup> [5], which is consistent with the  $Q^2$  range of the  $F_2^A/F_2^d$  data sets. Adjusting the input scale  $Q_0^2$  had a negligible effect below  $x_B \sim 0.7$  and adds, at most, a 5% systematic shift at  $x_B \sim 0.8$ .

We compared our model prediction up to  $x_B \sim 0.8$  when including and excluding the low  $W^2$  data, and took the difference between the two as a part of our systematic uncertainty. The two fitting procedures yielded very similar results up to  $x_B \sim 0.8$ , and thus including the low  $W^2$  data does not change our conclusions below  $x_B \sim 0.8$ . We note that, in particular, our  $F_2^p/F_2^d$  ratio saturates around  $x_B \sim 0.65$ , and thus, our conclusions are independent of the low  $W^2$  data. See top left panel of Figure 3.

Furthermore, while the nuclear DIS ratios  $F_2^A/F_2^d$  have been shown to be  $Q^2$  independent in the range of interest [7, 9],  $x \in [0.2, 0.8]$ ,  $Q^2 \in [2, 15]$ , our model also extracts a parameterization of  $F_2^p/F_2^d$ , which is much more sensitive to  $Q^2$  evolution. While our parameterization of  $F_2^p/F_2^d$  is constrained from all nuclear DIS data sets, it is also directly constrained by an input  $F_2^p/F_2^d$  data set from Ref. [5], which performs an evolution of global data sets of  $F_2^p/F_2^d$  to a common  $Q^2 = 12$  GeV<sup>2</sup>. This data set was used in our nominal fitting procedure, however, we also did a study to evolve the data set to a lower  $Q^2 = 5$  GeV<sup>2</sup>. Our evolution procedure used a simple scaling factor obtained following a parameterization of the  $Q^2$  dependence of  $F_2^p/F_2^d$  [10]. Repeating the fitting with the evolved  $F_2^p/F_2^d$  data set did not change our results below  $x_B \sim 0.8$ , as seen in the top right panel of Figure 3.

## EVOLVING $F_2^n/F_2^p$ TO THE MARATHON EXPERIMENT KINEMATICS

In Fig. 2 of the paper, we evolved extractions to the same value of  $Q^2$  based on the kinematics of the MARATHON experiment [11] (i.e.  $Q^2 = 14 \times x_B$  [GeV<sup>2</sup>]). The Arrington et al. prediction [12] was evolved self-consistently using their extracted  $Q^2$  dependence. The CT14 curve for  $F_2^n/F_2^p$  were constructed following the CJ15 framework (see below), and the PDFs were sampled at the corresponding MARATHON kinematics. The BONuS data was evolved to the MARATHON kinematics by using a  $Q^2$  parameterization of  $F_2^n/F_2^p$  [13]. Our model does not parameterize specific  $Q^2$  dependence, however, our model will be valid as some input  $Q_0^2$  scale, which corresponds to the  $Q^2$  range of the input data. As the data use covers the kinematic range of the MARATHON experiment, our model is valid to compare to their future results.

## FROM $F_2^n/F_2^p$ TO $d/u$ - COMPARISON TO PDF EXTRACTIONS (CT14)

Our model extracts  $F_2^n$  and  $F_2^p$  from measured experimental data, which are thus the “full-twist”, target-mass corrected (TMC), etc., structure functions. In Fig. 2 of the paper, we compare our model  $F_2^n/F_2^p$  (full-twist, TMC, etc.) to a few models, including CT14 and CJ15. The CJ15 prediction for  $F_2^n/F_2^p$  is given by Refs. [14, 15]. To build a corresponding  $F_2^n/F_2^p$  using CT14 PDFs, we follow the framework of CJ15 to build the corresponding structure functions from the individual parton distribution functions for CT14, while including target-mass corrections and higher-twist corrections [14] (all at MARATHON kinematics). Then, using Eqn. 1 of the paper, we consistently evolve all curves in Fig. 2 to predictions on  $d/u$ .

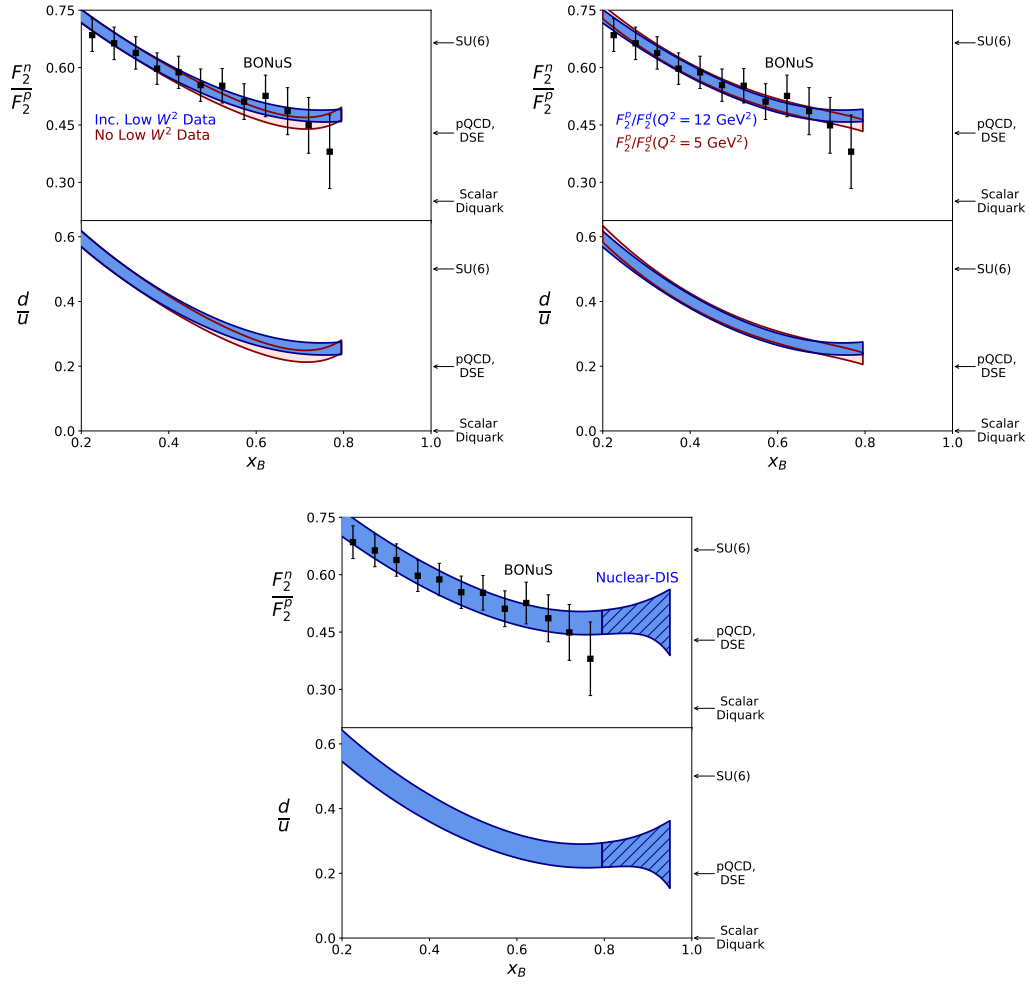

FIG. 3: Top left panel demonstrates the insensitivity of our conclusions to including/excluding the low  $W^2$  data. Top right panel demonstrates the  $Q^2$ -independence in our extraction our model range of interest. Bottom panel shows our model prediction 95% confidence bands.

### DEUTERON MODIFICATION TREATMENT

Our analysis also differs in its treatment of medium modification effects in the deuteron, which is largely driven by the heavy nuclei data. While our nominal model assumes self-consistency with the deuteron, we acknowledge that there is likely less modification due to short-range correlations as it's binding energy is small, SRCs make up roughly  $\sim 4\%$  of nuclear dynamics, etc.. As such, we performed a study where we allowed the strength of the modification in deuteron to be modulated by a parameter  $\lambda \in [0, 1]$ , and performed our global fit allowing this additional bounded parameter. This exercise resulted in identical extraction up to  $x_B \sim 0.8$  and only a very small variation above it. That means our equation for the deuteron structure function and EMC ratios become:

$$F_2^d = F_2^P + F_2^n + \lambda n_{SRC}^d (\Delta F_2^P + \Delta F_2^n)$$

$$\frac{2F_2^A}{AF_2^d} = \frac{2N}{A} + \frac{2(Z-N)}{A} \frac{F_2^P}{F_2^d} + \left( \frac{2n_{SRC}^A}{An_{SRC}^d} - \frac{2N\lambda}{A} \right) \frac{n_{SRC}^d (\Delta F_2^P + \Delta F_2^n)}{F_2^d} \quad (4)$$

We emphasize that this is not the same as changing definition in  $n_{SRC}^d$ , as that would affect how we can use our input data  $a_2(A/d) \equiv n_{SRC}^A/n_{SRC}^d$ .  $\lambda$  simply decreases modification contribution due to SRC in deuterium where now other mean-field effects may account for modification not as exaggerated in heavier nuclei.

While our fit converged on  $\lambda = 0.68 \pm 0.2$ , which is expected that modification is weaker, this did not change the results of our analysis below  $x_B \sim 0.8$  compared to our nominal model where we fix  $\lambda = 1$ , see Fig 4.

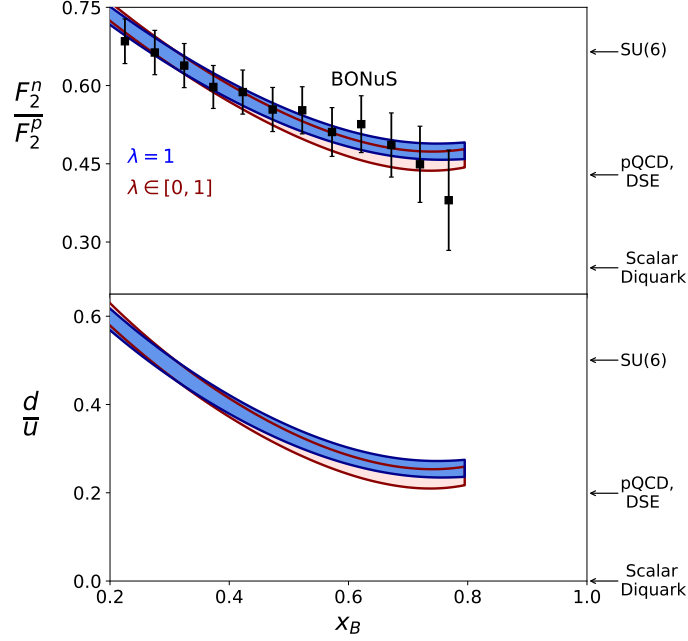

FIG. 4: Comparison of results when we allow  $\lambda$  as a bounded fit parameter between 0 and 1 and when we fix it to be 1. Within uncertainty, our results are the same below  $x_B \sim 0.8$ .

### COMPARING ISOSCALAR AND NON-ISOSCALAR PREDICTIONS

The Nuclear-DIS model as derived in the earlier section does not assume that the same modification for protons and neutrons, however, their relative contributions are indistinguishable in our model. All predictions from Kulagin and Petti (KP) are shown in their iso-scalar structure modification model (neutrons and protons modified the same) [6, 16, 17]. Three predictions are shown from a Tropiano et al. (TEMS) extraction [18] were described in the main text. We can benchmark all these models against the previously published  $^3\text{He}$  EMC ratio data set [4], and then compare how predictions look like for  $^3\text{H}$ , see Figure 5. Prediction comparisons for  $\mathcal{R}$  were shown in the paper, Figure 4.

While Fig. 3 in the main text assumed that  $a_2(^3\text{He}/d) = a_2(^3\text{H}/d)$ , see Fig 6 for the impact of slightly different values on predictions for  $F_2^{3\text{H}}/F_2^d$ .

### MODEL UNCERTAINTY IN $F_2^n/F_2^p$ EXTRACTION VIA $\mathcal{R}$ AND $F_2^{3\text{He}}/F_2^{3\text{H}}$

We estimate the model uncertainty of the extraction of  $F_2^n/F_2^p$  when extracted via:

$$\begin{aligned} \frac{F_2^n}{F_2^p} &= \frac{2\mathcal{R} - F_2^{3\text{He}}/F_2^{3\text{H}}}{2F_2^{3\text{He}}/F_2^{3\text{H}} - \mathcal{R}} \\ \mathcal{R} &= \frac{F_2^{3\text{He}}}{2F_2^p + F_2^n} \times \frac{F_2^p + 2F_2^n}{F_2^{3\text{H}}} \end{aligned} \quad (5)$$

by assuming various model predictions of  $F_2^{3\text{He}}/F_2^{3\text{H}}$  in combination with model predictions for  $\mathcal{R}$ . In the main text, in Figure 4 (right), we used our model prediction for  $F_2^{3\text{He}}/F_2^{3\text{H}}$  (grey bands in Figure 3) in combination with predictions for  $\mathcal{R}$  in order to extract  $F_2^n/F_2^p$  as outlined above. We reproduce this graph here in Figure 7 (left). We then assume a different model prediction for  $F_2^{3\text{He}}/F_2^{3\text{H}}$  and repeat the exercise. In Figure 7 (right), the TEMS-CJ prediction for  $F_2^{3\text{He}}/F_2^{3\text{H}}$  was used, in combination with other model predictions for  $\mathcal{R}$ .

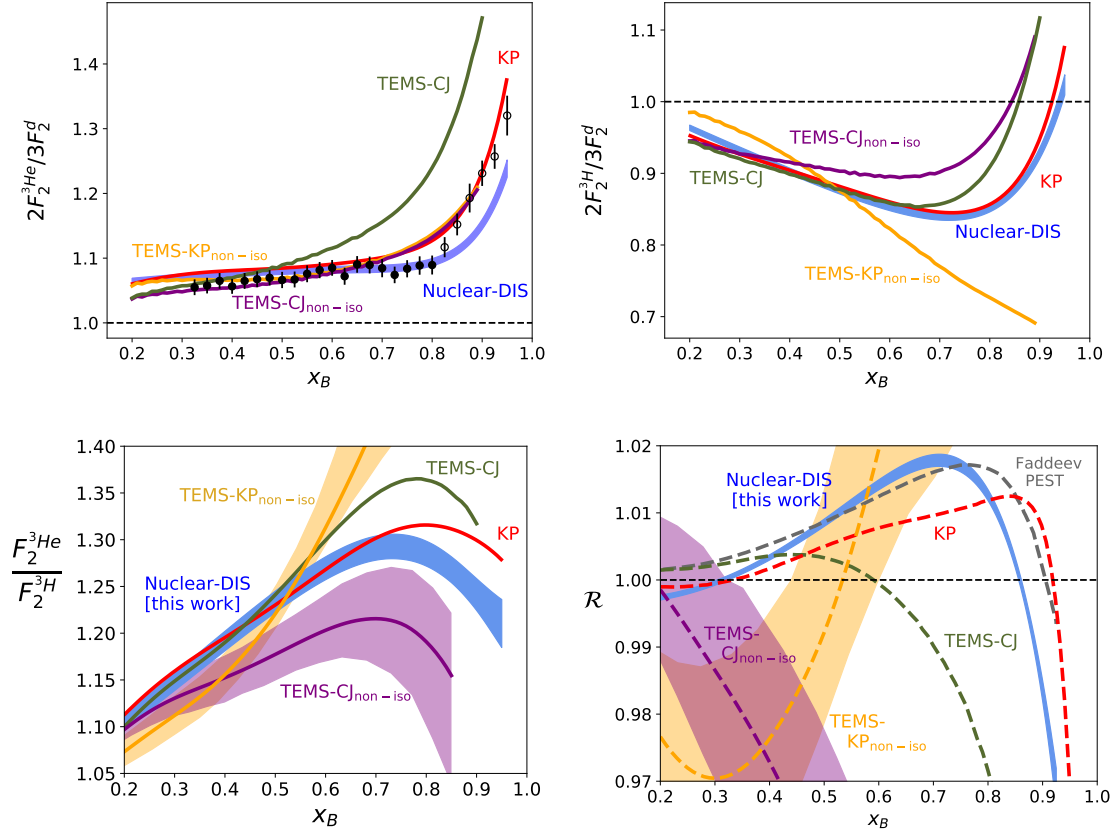

FIG. 5: (Top): Comparison of model predictions for EMC ratios in  $A = 3$  mirror-nuclei. When allowing for non-isoscalar offshell corrections, TEMS-CJ<sub>non-iso</sub> (purple) and TEMS-KP<sub>non-iso</sub> (orange) [18] seem to improve agreement to  ${}^3\text{He}$  data in comparison to fully isoscalar off-shell corrections (TEMS-CJ [green]). However, predictions for  ${}^3\text{H}$  diverge from other models at around  $x \sim 0.4$ . In particular, the TEMS-KP<sub>non-iso</sub> prediction does not follow the expected trend at high- $x$ , where fermi motion dominates the ratio. The Nuclear-DIS model is shown for a  $a_2({}^3\text{He}/d) = a_2({}^3\text{H}/d)$  prediction. (Bottom left):  $F_2^{3\text{H}}/F_2^d$  and  $F_2^{3\text{H}}/F_2^{3\text{He}}$  ratios for each model with systematic uncertainty for the two TEMS non-isoscalar predictions [18]. (Bottom right):  $\mathcal{R}$  predictions for each mode with systematic uncertainty for the two TEMS non-isoscalar predictions [18]. See text for details.

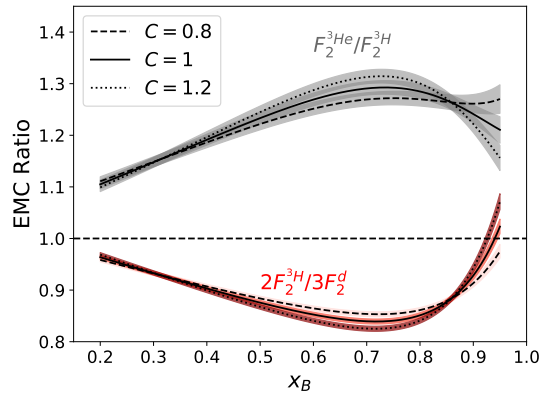

FIG. 6: Nuclear DIS analysis results for  $F_2^{3\text{H}}/F_2^d$  and  $F_2^{3\text{H}}/F_2^{3\text{He}}$  with different assumptions for  $n_{\text{SRC}}^{{}^3\text{H}} = C \times n_{\text{SRC}}^{{}^3\text{He}}$  for  $C = 0.8, 1, 1.2$

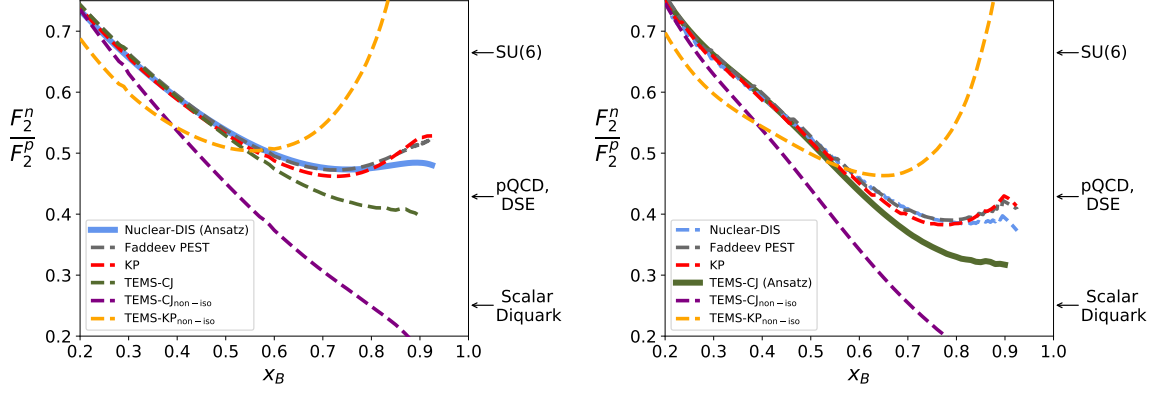

FIG. 7: Sensitivity on  $F_2^n/F_2^p$  extraction due to theoretical model uncertainty of  $\mathcal{R}$  when assuming a prediction (“Ansatz”) of  $F_2^{3\text{He}}/F_2^{3\text{H}}$ . In red is using a prediction of  $\mathcal{R}$  from KP [6, 16, 17]. Green, purple, and orange are using predictions of  $\mathcal{R}$  from a Tropiano et al. extraction [18] (see previous section for details). In gold is using a prediction of  $\mathcal{R}$  from Faddeev solution using PEST potential. [19]. In each curve in the left plot, the prediction of  $F_2^{3\text{He}}/F_2^{3\text{H}}$  is kept the same (taken from our Nuclear-DIS analysis), and in each curve in the right plot, the prediction of  $F_2^{3\text{He}}/F_2^{3\text{H}}$  is kept the same, as taken from TEMS-CJ analysis.

### STRUCTURE FUNCTION MODIFICATION WITH $nn$ , $pp$ , AND $np$ SRC PAIRS

Neglecting  $pp$  and  $nn$  SRC pairs does not change the UMF extracted from symmetric nuclei data and could change it only by a few percent for asymmetric nuclei. In symmetric nuclei, our model is still valid, assuming that the modification of protons (neutrons) is the same in  $np$  pairs and  $pp$  ( $nn$ ) pairs:

$$\begin{aligned} F_2^A &= ZF_2^p + NF_2^n + n_{SRC,np}^A (\Delta F_2^p + \Delta F_2^n) + 2(n_{SRC,nn}^A F_2^n + n_{SRC,pp}^A F_2^p) \\ F_2^A &= ZF_2^p + NF_2^n + n_{SRC,np}^A (\Delta F_2^p + \Delta F_2^n) + 2n_{SRC,np}^A (\Delta F_2^p + \eta \Delta F_2^n) \end{aligned} \quad (6)$$

where  $\eta = n_{SRC,nn}^A/n_{SRC,pp}^A$

Using deuterium (where  $n_{SRC,nn}^A = n_{SRC,pp}^A = 0$ ) again to form EMC ratios:

$$\begin{aligned} \frac{2F_2^A}{AF_2^d} &= \frac{2(Z-N)}{A} \frac{F_2^p}{F_2^d} + \frac{2N}{A} + \frac{\Delta F_2^p}{F_2^d/n_{SRC,np}^d} \left[ \frac{2n_{SRC,np}^A}{An_{SRC,np}^d} \left( 1 + 2\frac{n_{SRC,pp}^A}{n_{SRC,np}^d} \right) - \frac{2N}{A} \right] \\ &+ \frac{\Delta F_2^n}{F_2^d/n_{SRC,np}^d} \left[ \frac{2n_{SRC,np}^A}{An_{SRC,np}^d} \left( 1 + 2\eta \frac{n_{SRC,pp}^A}{n_{SRC,np}^d} \right) - \frac{2N}{A} \right] \end{aligned} \quad (7)$$

where previously, in our model assuming only  $np$  pairs,  $a_2(A/d) = 2n_{SRC,np}^A/An_{SRC,np}^d$ , now

$$a_2(A/d) = \frac{2n_{SRC,np}^A}{An_{SRC,np}^d} \left[ \frac{\left( 1 + \frac{\sigma_{ep}}{\sigma_{en}} \right) + \frac{2n_{SRC,pp}^A}{n_{SRC,np}^d} \left( \eta + \frac{\sigma_{ep}}{\sigma_{en}} \right)}{\left( 1 + \frac{\sigma_{ep}}{\sigma_{en}} \right)} \right] \quad (8)$$

Now we can see, for symmetric nuclei,  $\eta = 1$ , this formulation is identical to our model assumption, which was only based on  $np$  pairs, as for symmetric nuclei,  $a_2(A/d)$  simplifies to:

$$a_2(A/d) = \frac{2n_{SRC,np}^A}{An_{SRC,np}^d} \left[ 1 + \frac{2n_{SRC,pp}^A}{n_{SRC,np}^d} \right] \quad (9)$$

which means our Eqn. 7 reduces to:

$$\begin{aligned}
\frac{2F_2^A}{AF_2^d} &= \frac{2(Z-N)}{A} \frac{F_2^p}{F_2^d} + \frac{2N}{A} + \frac{\Delta F_2^p}{F_2^d/n_{SRC,np}^d} \left[ \frac{2}{A} \frac{n_{SRC,np}^A}{n_{SRC,np}^d} \left( 1 + 2 \frac{n_{SRC,pp}^A}{n_{SRC,np}^A} \right) - \frac{2N}{A} \right] \\
&\quad + \frac{\Delta F_2^n}{F_2^d/n_{SRC,np}^d} \left[ \frac{2}{A} \frac{n_{SRC,np}^A}{n_{SRC,np}^d} \left( 1 + 2 \frac{n_{SRC,pp}^A}{n_{SRC,np}^A} \right) - \frac{2N}{A} \right] \\
\frac{2F_2^A}{AF_2^d} &= \frac{2(Z-N)}{A} \frac{F_2^p}{F_2^d} + \frac{2N}{A} + \frac{\Delta F_2^p}{F_2^d/n_{SRC,np}^d} \left[ a_2(A/d) - \frac{2N}{A} \right] + \frac{\Delta F_2^n}{F_2^d/n_{SRC,np}^d} \left[ a_2(A/d) - \frac{2N}{A} \right] \\
\frac{2F_2^A}{AF_2^d} &= \frac{2(Z-N)}{A} \frac{F_2^p}{F_2^d} + \frac{2N}{A} + \frac{\Delta F_2^p + \Delta F_2^n}{F_2^d/n_{SRC,np}^d} \left( a_2(A/d) - \frac{2N}{A} \right) \\
\frac{2F_2^A}{AF_2^d} &= \frac{2(Z-N)}{A} \frac{F_2^p}{F_2^d} + \frac{2N}{A} + f_{\text{univ}} \left( a_2(A/d) - \frac{2N}{A} \right)
\end{aligned} \tag{10}$$

which is indistinguishable from our current model considering only  $np$  pairs, except the definition of  $a_2(A/d)$  has evolved.

- 
- [1] B. Schmookler *et al.* (CLAS), Nature **566**, 354 (2019).
  - [2] B. Carpenter, A. Gelman, M. Hoffman, D. Lee, B. Goodrich, M. Betancourt, M. Brubaker, J. Guo, P. Li, and A. Riddell, Journal of Statistical Software, Articles **76**, 1 (2017).
  - [3] S. D. Team, “Pystan: the python interface to stan, version 2.17.1.0,” <http://mc-stan.org> (2018).
  - [4] J. Seely *et al.*, Phys. Rev. Lett. **103**, 202301 (2009).
  - [5] J. Arrington, F. Coester, R. J. Holt, and T. S. H. Lee, J. Phys. **G36**, 025005 (2009), arXiv:0805.3116 [nucl-th] .
  - [6] S. A. Kulagin and R. Petti, Phys. Rev. **C82**, 054614 (2010), arXiv:1004.3062 [hep-ph] .
  - [7] J. Gomez *et al.*, Phys. Rev. D **49**, 4348 (1994).
  - [8] J. Arrington, R. Ent, C. Keppel, J. Mammei, and I. Niculescu, Phys. Rev. **C73**, 035205 (2006).
  - [9] J. Seely *et al.*, Phys. Rev. Lett. **103**, 202301 (2009).
  - [10] L. Whitlow *et al.*, Phys. Lett. **B282**, 475 (1992).
  - [11] G. G. Petratos *et al.*, Jefferson Lab PAC37 Proposal (2010), experiment E12-10-103.
  - [12] J. Arrington, J. G. Rubin, and W. Melnitchouk, Phys. Rev. Lett. **108**, 252001 (2012), arXiv:1110.3362 [hep-ph] .
  - [13] P. Amaudruz *et al.* (The New Muon Collaboration (NMC)), Nucl. Phys. **B371**, 3 (1992).
  - [14] A. Accardi, L. T. Brady, W. Melnitchouk, J. F. Owens, and N. Sato, Phys. Rev. **D93**, 114017 (2016), arXiv:1602.03154 [hep-ph] .
  - [15] A. Accardi, (private communication).
  - [16] S. Kulagin and R. Petti, Nuclear Physics A **765**, 126 (2006).
  - [17] S. A. Kulagin and R. Petti, (private communication).
  - [18] A. Tropicano, J. Ethier, W. Melnitchouk, and N. Sato, Phys. Rev. **C99**, 035201 (2019), arXiv:1811.07668 [hep-th] .
  - [19] I. R. Afnan, F. R. P. Bissey, J. Gomez, A. T. Katramatou, S. Liuti, W. Melnitchouk, G. G. Petratos, and A. W. Thomas, Phys. Rev. **C68**, 035201 (2003), arXiv:nucl-th/0306054 [nucl-th] .
